# Supplementary material for: A Closer Look at Knowledge Distillation in Spiking Neural Network Training
Source: arXiv:2511.06902 source file (2025-11-14)
Supplement: Supplementary file 1 [file 12_appendix.tex]

% \section{Rebuttal}
% \input{_rebuttal}
% \noindent We sincerely appreciate invaluable feedback from the reviewers and will incorporate all of it in the revision.
% %% 

% % \noindent [\textcolor{red}{qtNG}]
% % \textbf{Novelty for CAM-SAM Distillation}.

% % \noindent [\textcolor{red}{qtNG},\textcolor{orange}{XEyM}]
% % \textbf{Novelty for Noise}.

% \noindent [\textcolor{magenta}{qtNG},\textcolor{orange}{XEyM}] 
% % 论文忽略了分析SAMD引入的计算开销和训练时间影响
% \textbf{SAMD strategy training overhead.}

% % 我们分析了训练过程中的计算开销，结果如图~\ref{ab1}所示。在 ImageNet 上，我们的方法能耗略高于 KDSNN，但明显低于 BKDSNN，尤其在ResNet50的架构上。鉴于其在性能上的优势，我们认为这一额外开销是合理且可接受的。
% We analyze the computational overhead during training, as shown in Fig.~\ref{overhead}. 
% On ImageNet, our method incurs slightly higher energy consumption than KDSNN but 
% is significantly lower than BKDSNN, 
% especially with the ResNet50. 
% Given its performance advantage, 
% we consider this additional overhead reasonable and acceptable.
% \input{figs/overhead_and_ablation}
% \noindent [\textcolor{magenta}{qtNG},\textcolor{cyan}{uVUV}]
% \textbf{The consistency in experimental results.}
% % Thank you for your suggestion. 我们展示了在同一架构下的消融实验，如图~\ref{overhead} Right 所示。
% Thank you for your suggestion. 
% We show the ablation experiments under the same architecture, 
% as shown in the right of Fig.~\ref{overhead} (a) (b) (c).

% \noindent [\textcolor{magenta}{qtNG}] \textbf{The effect of saliency scaled maps.} 
% % 图3(e)展示了我们对 saliency scaled 在训练中作用的消融实验。我们发现，在训练初期，未使用 saliency scaled 的方法收敛较快；但在后期，引入 saliency scaled 的方法表现出更强的鲁棒性。
% % 因此，我们认为 saliency scaled 在整个训练过程中起到了关键作用。
% We conduct an ablation study on the effect of saliency scaled maps in training, as shown in Fig.~\ref{overhead} (d).
% We find that the method without saliency scaled converges faster in the early training stage,
% but the method with saliency scaled exhibits stronger robustness in the later stage.
% Thus, we believe that saliency scaled plays a key role throughout the training process.

% \input{figs/logits_feature_sparse}
% \noindent [\textcolor{magenta}{qtNG},\textcolor{orange}{XEyM}] \textbf{The novelty of CKDSNN.}

% \input{figs/different_work_compare}
% \noindent [\textcolor{magenta}{qtNG}] \textbf{The SOTA comparison with Enof.}

% \noindent [\textcolor{orange}{XEyM}]


% \begin{table}[t]
% \footnotesize
% \vspace{-3ex}
% \caption{\label{Table3} Ablation study on the saliency-scaling manners in SAMD. The ResNet-18 and SEW-ResNet-18 are used as the teacher and student models, respectively.}
% \vspace{-1ex}
% % \begin{minipage}[t]{0.45\textwidth}
% \centering
% \resizebox{\linewidth}{!}{
% \begin{tabular}{c|>{\centering}p{1.2cm}|>{\centering}p{1.2cm}|>{\centering}p{1.2cm}|c}
% \toprule
%  & \makecell{Min-Max } & \makecell{Z-score } & \makecell{L2-norm } & \makecell{\textbf{Softmax}} \\  \midrule
%  % &  &  &  &  & &  \\  \midrule
% CIFAR-10
% & 89.33 & 88.45 & 89.06 & \textbf{91.22} \\ \midrule
% CIFAR-100
% & 73.01 & 72.38 & 73.50 & \textbf{75.31} \\ 
% \bottomrule
% \end{tabular}
% }
% % \end{minipage}%
% \vspace{-1.8ex}
% \end{table}

% 我们注意到审稿人提到不同表格中的实验结果之间存在不可交叉验证的现象。
% 实际上，这些表格所展示的是在不同实验设置 （不同的教师模型、学生模型）下获得的结果，并非同一条件下重复实验的输出。
% 因此，它们之间的不一致性并不意味着实验存在问题，而是反映了模型性能在不同配置下仍能保持稳定或具有一定适应性 的变化趋势。
% 为了进一步增强实验结果之间的可比性和说服力，我们在相同的教师和学生模型下设计了一组控制变量实验，
% 确保在除目标方法外的其他条件完全一致的情况下进行性能对比 。

% Several tables contain results that cannot be cross-verified against one another, raising concerns about experimental rigor.

% SAMD relies on the ANN’s class activation maps, so any localization errors may be transferred to the SNN.

% 【1】Lack of novelty. Distillation using saliency maps is not a new strategy in machine learning, e.g. [1] and [2] use CAM to distill ANNs, and this paper simply transplants it to SNNs. In addition, adding noise to the output of the student model has also been studied in ANN [3].

% 【2】 The effectiveness of the proposed method lacks theoretical justification, and the authors should explain the unique role of their transplantation of the ANN method to the SNN domain in conjunction with spike properties.

% 【3】 Using CAM to obtain saliency maps for the teacher ANN model will increase the training overhead, and it is suggested that the authors provide a training overhead analysis of their method.

% The method proposed in this paper includes hyperparameters such as the coefficients of distillation loss (
%  and 1.0 for 
%  in Eq. 8) and noise intensity (
%  in Eq. 6), and the authors should analyze the influence of these hyperparameters on the performance.

% The comparative methods in the paper are inadequate and lack up-to-date and representative methods. For example, [4] used ANN to distill SNNs without computing CAM maps to achieve 82.43\% accuracy on CIFAR100 using ResNet19 in 2 time steps, exceeding the accuracy reported in this paper. Authors should not ignore these related efforts in their comparisons.

% Why don't the authors use a consistent architecture for the ablation experiments in Tables 3, 4, and 6 in the Experiments section? In addition, I note that the use of ResNet-18 in Table 4 achieved only 91.22\% accuracy on CIFAR10, which is significantly lower than the existing SNNs.

% What is the effect of not normalizing the saliency maps with the softmax function when using SAMD, i.e. is this step necessary?



% review3
%  【4】 Unjustified Loss of Channel Information in Feature Alignment: SAMD aligns features using CAMs, reducing them to 2D spatial maps and discarding channel details. The paper lacks justification for ignoring potentially valuable channel-specific teacher patterns. Evidence is required if the authors claim channel information is negligible due to SNN sparsity.

% 【5】Unsupported Claim of "Sharper" SNN Logits: The assertion that SNN output logits are sparser and more peaked than ANN logits lacks quantitative evidence. The paper needs supporting statistics or visualizations to validate this claim.

%【6】 Limited Novelty and Missing Experiments for Noise-Based KD (NLD): Prior work [1] explored noise in KD, notably finding “a noisy teacher is more helpful than a noisy student”, whereas NLD adds noise to the student. This raises two issues:

% Novelty: Given existing noise-based KD approaches, the authors should clarify how NLD differs from prior work; otherwise, its only novelty may be the application to SNNs.
% Exploration of Teacher-side Noise: Given prior findings [1], omitting experiments where noise is added to the teacher's logits is an oversight.

%% 审稿人2 
% SAMD relies on the ANN’s class activation maps, so any localization errors may be transferred to the SNN.

% \label{sec:rebuttal_section}
% (1) Training curves for ImageNet-1k dataset.
% (2) Evaluation of the proposed method on Neuromorphic datasets.
% (3) Various ablation studies e.g., the effect of different spiking transformer architectures.
%

% Supplementary material goes here.
